# Supplementary material for: Efficient Optimization for Rank-based Loss Functions
Source: arXiv:1604.08269 source file (2018-02-28)
Supplement: Supplementary file 1 [file additional.tex]

The computation of the optimal interleaving rank for a particular negative
sample requires us to maximize the discrete function $f_j(i)$ over the domain $i \in \{1,\cdots,|{\cal P}|\}$ (or possibly its subdomain). Yue {\em et al.\ }\cite{yuesigir07}
use a simple linear algorithm for this step, which takes $O(|{\cal P}|)$ time. In contrast, we propose a more efficient algorithm to maximize
$\delta_j(\cdot)$, which exploits the special structure of this discrete function. This will not bring improvement in the worst-case complexity but it adds another speed-up and is interesting conceptually.

Before we describe our efficient algorithm in detail, we require the definition of a unimodal function. A discrete function $f:\{1,\cdots,p\} \leftarrow \mathbb{R}$
is said to be unimodal if and only if there exists a $k \in \{1,\cdots,p\}$ such that
\begin{eqnarray}
&&f(i) \leq f(i+1), \forall i \in \{1,\cdots,k-1\}, \nonumber \\
&&f(i-1) \geq f(i), \forall i \in \{k+1,\cdots,p\}.
\end{eqnarray}
In other words, a unimodal discrete function is monotonically non-decreasing in the interval $[1,k]$ and monotonically non-increasing in the interval $[k,p]$.
The maximization of a unimodal discrete function over its domain $\{1,\cdots,p\}$ simply requires us to find the index $k$ that satisfies the above
properties. The maximization can be performed efficiently, in $O(\log(p))$ time, using binary search.

We are now ready to state the main result that allows us to compute the optimal interleaving rank of a negative sample efficiently.
\begin{proposition}\label{prop:unimodal}\setcounter{foo}{\value{theorem}}
%\item 
The discrete function $f_j(i)$, induced by $\Delta_{AP}$, is unimodal in the domain $\{1,\cdots,p\}$, where
$p = \min\{|{\cal P}|,j\}$.
%\label{prop:unimodal}
\end{proposition}

The proof of the above proposition is provided in Appendix \ref{sec:lossprops}.

\begin{algorithm}[h]
\caption{\em Efficient search for the optimal interleaving rank of a negative sample.} \label{alg2}
\SetAlgoLined
\DontPrintSemicolon

\nonl 
{\bf Input:} $\{f_j(i),i=1,\cdots,|{\cal P}|\}$. \\
\vspace{-10pt}\; 

$p = \min\{|{\cal P}|,j\}$\;
Compute an interleaving rank $i_1$ as
\begin{equation}
i_i = \argmax_{i \in \{1,\cdots,p\}} f_j(i).
\end{equation}\vspace{-10pt}\;
Compute an interleaving rank $i_2$ as
\begin{equation}
i_2 = \argmax_{i \in \{p+1,\cdots,|{\cal P}|\}} f_j(i).
\end{equation}\vspace{-10pt}\;
Compute the optimal interleaving rank $opt_j$ as
\begin{equation}
opt_j = \left\{
\begin{array}{cl}
i_1 & \mbox{if } f_j(i_1) \geq f_j(i_2), \\
i_2 & \mbox{otherwise}.
\end{array}
\right.
\end{equation}

\end{algorithm}
Using the above proposition, the discrete function $f_j(i)$ can be optimized over the domain $\{1,\cdots,|{\cal P}|\}$ efficiently
as described in Algorithm~\ref{alg2}. Briefly, our efficient search algorithm finds
an interleaving ranking $i_1$ over the domain $\{1,\cdots,p\}$, where
$p$ is set to $\min\{|{\cal P}|,j\}$ in order to ensure that the function $f_j(\cdot)$ is unimodal (step 2 of Algorithm~\ref{alg2}).
Since $i_1$ can be computed using binary search, the computational complexity of this step is $O(\log(p))$.
Furthermore, we find an interleaving ranking $i_2$ over the domain $\{p+1,\cdots,|{\cal P}|\}$ (step 3 of Algorithm~\ref{alg2}).
Since $i_2$ needs to be computed using linear search, the computational complexity of this step is $O(|{\cal P}|-p)$ when $p < |{\cal P}|$ and $0$ otherwise.
The optimal interleaving ranking $opt_j$ of the negative sample ${\bf x}_j$ can then be computed by comparing the values of
$f_j(i_1)$ and $f_j(i_2)$ (step 4 of Algorithm~\ref{alg2}).

Note that, in a typical training data set, the negative samples significantly outnumber the positive samples, that is, $|{\cal N}| \gg |{\cal P}|$.
For all the negative samples ${\bf x}_j$ where $j \geq |{\cal P}|$, $p$ will be equal to $|{\cal P}|$. Hence, the maximization of $f_j(\cdot)$ can
be performed efficiently over the entire domain $\{1,\cdots,|{\cal P}|\}$ using binary search in $O(\log(|{\cal P}|))$ as opposed to the
$O(|{\cal P}|)$ time suggested in~\cite{yuesigir07}.
